# Supplementary material for: Thermal effects on the lifetime of evaporating drops on fibers
Source: arXiv:2412.09336 source file (2024-12-12)

(a)

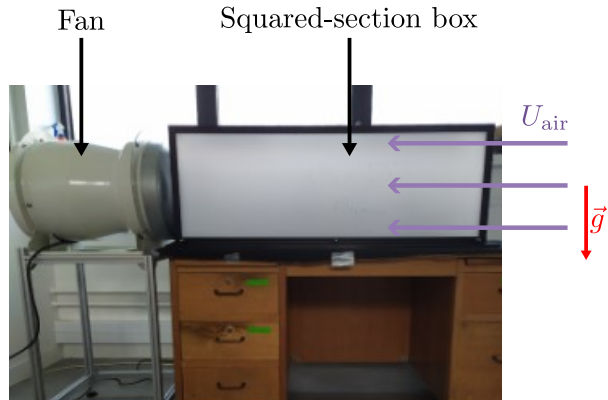

(b)

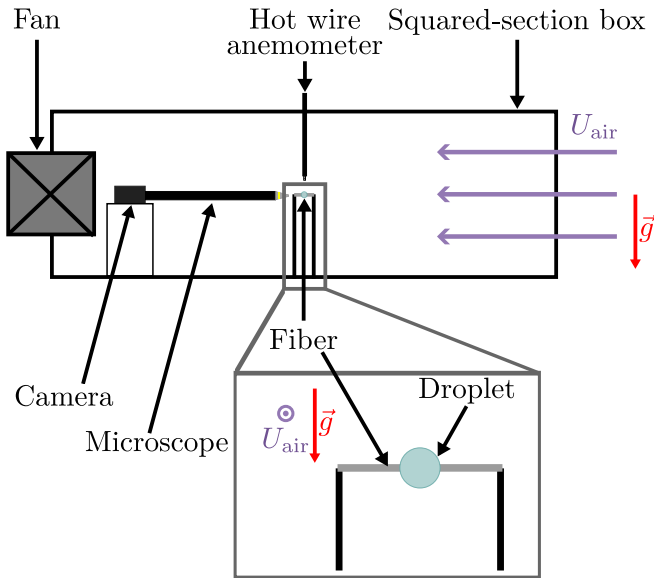

Supplement: Supplementary file 1 [file SM_scheme_wind_tunnel.pdf]
